# Supplementary material for: Resource Allocation in Multi-armed Bandit Exploration: Overcoming Sublinear Scaling with Adaptive Parallelism
Source: arXiv:2011.00330 source file (2021-06-05)
Supplement: Supplementary file 1 [file old_appendix.tex]

% \kkcomment{I have some suggestions below on how to write up the proofs.}
% \kkcomment{Are you familiar with the begingroup, allowdisplaybreaks, endgroup commands?
% This will allow you to carry an equation over to the next page and avoid formatting issues.
% I have used it in some examples below. Also, I am above 8 pages but this could be an issue with
% my compiler.}

% \insertprethmspacing
% \begin{theorem}
% \label{thm:fixed_confidence_runtime}
% % Define $g(x) = \lambda(1/x)$. Let $g$ be a non-decreasing, concave function where $g(0) = 0$. With probability at least $1 - \delta$,
% Assume $\lambda$ satisfies the assumptions in Section~\ref{sec:environment}.
% Let $\beta \in (1,n]$.
% Let $\omega = \sqrt{\delta/(6n)}$ and define $\bar{N}_i :=
% 1 + \left\lfloor 64\Delta_i^{-2}\log((2/\omega)\log_2(192\Delta_i^{-2}/\omega))\right\rfloor$
% $\forall i \in [n]$.
% Let $\Tcal_2$ be as defined in~\eqref{eqn:dp}.
% With probability at least $1 - \delta$,
% Algorithm~\ref{alg:fixed_confidence} outputs the best arm and the total execution time of the
% algorithm $T$ satisfies,
% \begingroup
% \allowdisplaybreaks
% \begin{align*}
%     T &\;\leq\; 4\frac{\beta^{3 + 4\sqrt{\log_\beta(n)}}}{\beta - 1}
%         \Tcal_2\left( \{\bar{N}_i\}_{i=2}^n\right) \\
%     &\leq 512\frac{\beta^{3+4\sqrt{\log_\beta(n)}}}{\beta - 1}
%     % &\hspace{0.4in}
%     \left(\log\left(\frac{2}{\omega}\log_2\left(\frac{192}{\Delta^2_2\omega}\right)\right)\lor \frac{1}{64}\right)T^\star
% %     &\;\leq\; 4\frac{\beta^{3 + 4\sqrt{\log_\beta(n)}}}{\beta - 1}\scalefunc(n) \;\;+ \\
% %      &\hspace{0.4in}
% % 256\log\left(\frac{2}{\omega}\log_2\left(\frac{192}{\Delta_i^{2}\omega}\right)\right)
% %         \frac{\beta^{3 + 4\sqrt{\log_\beta(n)}}}{\beta - 1} \Tstar.
% \end{align*}
% \endgroup
% % \kkcomment{fix this.}
% \end{theorem}

% \insertprethmspacing
% \begin{theorem}
% Fix $\muone>\mutwo\geq\dots\geq \mun$.
% Let $\Deltai$ be as defined in~\eqref{eqn:Deltai} for these $\{\mui\}_i$ values,
% and $\Tstar$ be as defined in~\eqref{eqn:Tstar} for these $\{\Deltai\}_i$ values.
% Assume $\lambda$ satisfies the assumptions in Section~\ref{sec:environment}, and additionally 
% for some $\alpha_1$,
% $\alpha_1 m \leq \scalefunc(m)\;
% \text{for all } m\geq 1.$
% Then, there exists a set of distributions
%  $\theta\in\Theta$ whose ordered mean values are $\{\mui\}_i$ as defined above
% % and (ii) a scaling function $\scalefunc$,
% such that for all $\delta\leq 0.15$,
% \[
% \inf_{A\in\Acaldelsf} \EE[T(A,\theta)] \geq 2 c_\scalefunc
% \log\left(\frac{1}{2.4\delta} \right)\Tstar.
% \]
% Here, $c_\scalefunc$ is a constant that depends only on $\scalefunc$.
% \label{thm:fixed_confidence_lowerbound}
% \end{theorem}

% \insertprethmspacing
% \begin{theorem}\label{thm:fixed_budget_error_prob}
% Assume $\scalefunc$ satisfies the assumptions in Section~\ref{sec:environment}.
% Suppose Algorithm~\ref{alg:fixed_budget} is run for some
% $k \in \NN_+$. Then, Algorithm~\ref{alg:fixed_budget} identifies the best arm in time at most
% $T$ with probability at least:
% \begin{align}
%     1 -  3\lceil\log_2(n)\rceil \exp \left(-\frac{nx(k)}{8H_2}\right)\label{eq:fb_success_prob}
% \end{align}
% where $H_2 = \max_{i\neq 1} i\Delta^{-2}_i$ and $\Deltai$ is as defined in~\eqref{eqn:Deltai}.
% \end{theorem}
